# Supplementary material for: Predicting rigidity and connectivity percolation in disordered particulate networks using graph neural networks
Source: arXiv:2411.14159 source file (2025-03-28)
Supplement: Supplementary file 1 [file Supplementary_Material.pdf]

**Supplementary Information for 'Predicting rigidity and connectivity percolation in disordered particulate networks using graph neural networks', author D.A. Head.**

*Prepared November 21, 2024*

# S1 Training and meta-parameter ranges

To estimate suitable ranges for the meta-parameters, the data sets with the smallest number of samples (lattice size $L = 100$ for the lattice data; $N = 10^4$ particles for the off-lattice data) were selected, preliminary runs were used to identify reasonable meta-parameters, and then the maximum number of epochs and the number of folds were varied as shown in Fig. S1. From this data, it is evident that there was at most minimal benefit from allowing more than 200 epochs of training, or to use more than $k \approx 4$ folds.

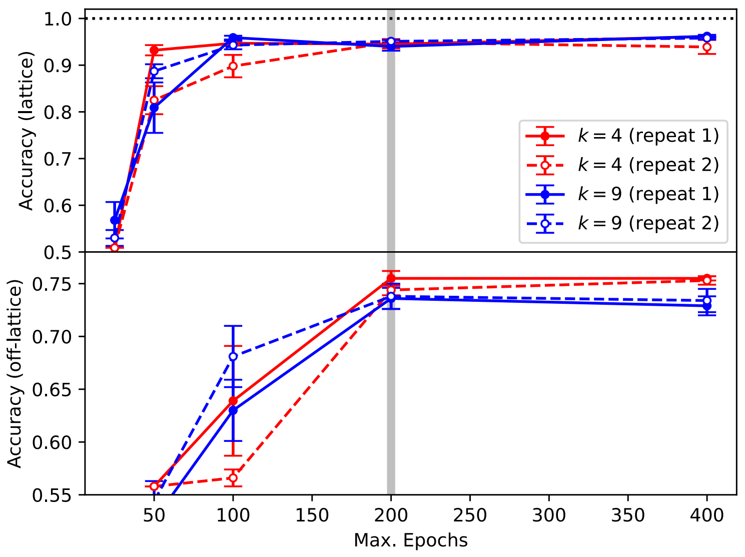


Figure S1: Final evaluation accuracy achieved against the maximum number of training epochs for rigidity classification on the $L = 100$ lattice data (top) and the $N = 10^4$ off-lattice data (bottom), for the given $k$-fold cross validation, each with two repeats. Error bars are the standard error of the mean across folds. The meta-parameters were $\ell_r = 3 \times 10^{-3}$, $n_{\text{batch}} = 32$, $n_H = 3$, $n_C = 15$ and $K = 3$.

Reasonable ranges for the meta-parameters were estimated by varying each from the values used in Fig. S1. The variation of the accuracy is shown in Fig. S2. For the lattice data, the learning rate $\ell_r$ and batch size achieved peak accuracy at $10^{-2}$ and 32 respectively. For the remaining parameters there was no clear optimum for $K > 1$, $n_H > 1$, and $n_C > 5$. For the off-lattice data in the same figure, the preferred learning rate and batch size were $\ell_r = 3 \times 10^{-3}$ and 32, with again minimal variation for the remaining parameters beyond the lowest values tested.

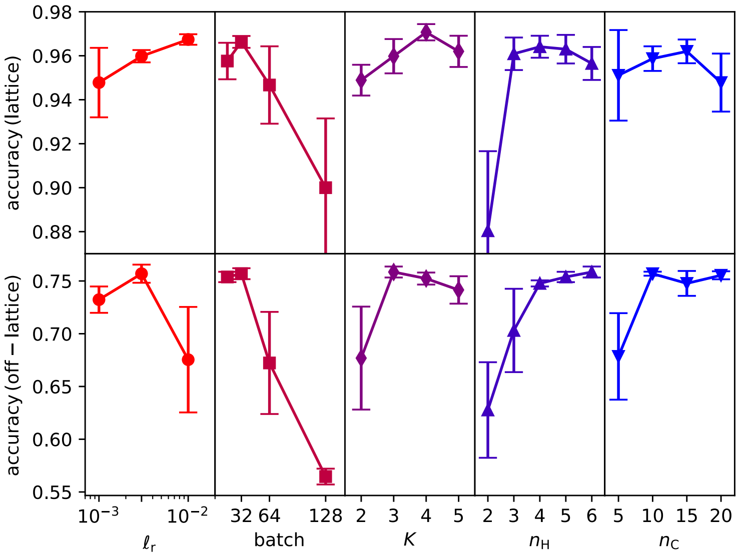


Figure S2: Accuracies for varying each parameter independently from the initial values learning rate $\ell_r = 3 \times 10^{-3}$, $n_{batch} = 32$, $K = 3$, $n_H = 3$ and $n_C = 15$, with $k = 5$–fold cross validation. The top row corresponds to the lattice data ($L = 100$), and the bottom row to the off-lattice data ($N = 10^4$). For both rows, the points for $\ell_r = 3 \times 10^{-2}$, $\ell_r = 10^{-1}$, $K = 1$, and $n_H = 1$, are not shown as they achieved minimal or no training.

# S2 Varying meta-parameters

Based on the results of Fig S2, each combination of $K = 2$ or 4, $n_H = 2$ or 4, and $n_C = 10$ or 20, was systematically evaluated and the accuracies presented in Tables S1–S4 for both lattice and off-lattice data, and rigidity and connectivity percolation problems.

# S3 Model variations

The maximum accuracies achieved for varying the model and the graph data are presented in Table S5 for off-lattice data, for both rigidity and connectivity classification problems. The equivalent for off-lattice data is given in Table S6.

# References

[1] `github.com/pyg-team/pytorch_geometric`.

[2] Michaël Defferrard, Xavier Bresson, and Pierre Vandergheynst. Convolutional neural networks on graphs with fast localized spectral filtering. *Advances in Neural Information Processing Systems*, 2016.

| $L$ | $K$ | $n_{\mathrm{H}}$ | $n_{\mathrm{C}}$ | Accuracy | $L$ | $K$ | $n_{\mathrm{H}}$ | $n_{\mathrm{C}}$ | Accuracy | $L$ | $K$ | $n_{\mathrm{H}}$ | $n_{\mathrm{C}}$ | Accuracy |
|---|---|---|---|---|---|---|---|---|---|---|---|---|---|---|
| 20 | 2 | 2 | 10 | 0.847(3) | 50 | 2 | 2 | 10 | 0.932(3) | 100 | 2 | 2 | 10 | 0.955(9) |
| | | | 20 | 0.862(8) | | | | 20 | 0.935(4) | | | | 20 | 0.952(5) |
| | | 4 | 10 | 0.88(2) | | | 4 | 10 | 0.925(6) | | | 4 | 10 | 0.960(3) |
| | | | 20 | 0.82(2) | | | | 20 | 0.927(7) | | | | 20 | 0.951(6) |
| | **4** | **2** | **10** | **0.926(3)** | | **4** | **2** | 10 | 0.942(5) | | **4** | **2** | 10 | 0.95(1) |
| | | | 20 | 0.913(9) | | | | **20** | **0.955(4)** | | | | **20** | **0.972(5)** |
| | | 4 | 10 | 0.83(5) | | | 4 | 10 | 0.938(6) | | | 4 | 10 | 0.95(1) |
| | | | 20 | 0.79(7) | | | | 20 | 0.68(9) | | | | 20 | 0.7(1) |

Table S1: Evaluation accuracies for lattice rigidity percolation data varying the meta-parameters $K$, $n_{\mathrm{H}}$ and $n_{\mathrm{C}}$, for learning rate $\ell_{\mathrm{r}} = 10^{-2}$ and a batch size of 32. Numbers in brackets give the estimated error in final digit (standard error over $k = 5$ folds). Meta-parameters used for subsequent analysis in the main text are highlighted in bold.

| $L$, $o_1$ | $K$ | $n_{\mathrm{H}}$ | $n_{\mathrm{C}}$ | Accuracy | $L$, $o_1$ | $K$ | $n_{\mathrm{H}}$ | $n_{\mathrm{C}}$ | Accuracy | $L$, $o_1$ | $K$ | $n_{\mathrm{H}}$ | $n_{\mathrm{C}}$ | Accuracy |
|---|---|---|---|---|---|---|---|---|---|---|---|---|---|---|
| 20, 3 | 2 | 2 | 10 | 0.816(2) | 50, 6 | 2 | 2 | 10 | 0.899(2) | 100, 14 | 2 | 2 | 10 | 0.927(1) |
| | | | 20 | 0.815(1) | | | | 20 | 0.896(2) | | | | 20 | 0.926(1) |
| | | 4 | 10 | 0.817(4) | | | 4 | 10 | 0.904(2) | | | 4 | 10 | 0.922(1) |
| | | | 20 | 0.811(4) | | | | 20 | 0.899(3) | | | | 20 | · · · |
| | **4** | 2 | 10 | 0.825(2) | | **4** | 2 | 10 | 0.906(2) | | **4** | 2 | 10 | 0.922(1) |
| | | | 20 | 0.832(2) | | | | 20 | 0.901(2) | | | | 20 | 0.921(2) |
| | | **4** | **10** | **0.833(2)** | | | **4** | **10** | **0.910(2)** | | | **4** | **10** | **0.929(2)** |
| | | | 20 | 0.81(1) | | | | 20 | 0.903(8) | | | | 20 | · · · |

Table S2: Evaluation accuracies for lattice connectivity percolation data, with $L$ the lattice size and $o_1$ the factor by which class 1 was oversampled to give approximate class balance (see main text). The '· · ·' for $L = 100$ denote that training was not possible on the production system.

| $N$ | $K$ | $n_{\mathrm{H}}$ | $n_{\mathrm{C}}$ | Accuracy | $N$ | $K$ | $n_{\mathrm{H}}$ | $n_{\mathrm{C}}$ | Accuracy | $N$ | $K$ | $n_{\mathrm{H}}$ | $n_{\mathrm{C}}$ | Accuracy |
|---|---|---|---|---|---|---|---|---|---|---|---|---|---|---|
| $10^2$ | 2 | 2 | 10 | 0.796(2) | $10^3$ | 2 | 2 | 10 | 0.845(3) | $10^4$ | 2 | 2 | 10 | 0.554(1) |
| | | | 20 | 0.802(4) | | | | 20 | 0.850(4) | | | | 20 | 0.554(1) |
| | | 4 | 10 | 0.842(3) | | | 4 | 10 | 0.854(1) | | | 4 | 10 | 0.60(4) |
| | | | 20 | 0.844(2) | | | | 20 | 0.852(3) | | | | 20 | 0.746(1) |
| | **4** | 2 | 10 | 0.822(3) | | **4** | 2 | 10 | 0.863(5) | | **4** | 2 | 10 | 0.61(4) |
| | | | 20 | 0.828(5) | | | | 20 | 0.865(4) | | | | 20 | 0.65(4) |
| | | **4** | 10 | 0.849(3) | | | **4** | 10 | 0.859(5) | | | **4** | 10 | 0.743(4) |
| | | | **20** | **0.870(4)** | | | | **20** | **0.868(7)** | | | | **20** | **0.748(7)** |

Table S3: Evaluation accuracies for off-lattice rigidity percolation data varying the meta-parameters $K$, $n_{\mathrm{H}}$ and $n_{\mathrm{C}}$, for learning rate $\ell_{\mathrm{r}} = 3 \times 10^{-3}$ and a batch size of 32. Digits in brackets give the estimated error in final digits (standard error over the $k = 5$ folds). Meta-parameters used for subsequent analysis are highlighted in bold.

| $N$, $(o_1, o_2)$ | $K$ | $n_{\mathrm{H}}$ | $n_{\mathrm{C}}$ | Acc. | $N$, $(o_1, o_2)$ | $K$ | $n_{\mathrm{H}}$ | $n_{\mathrm{C}}$ | Acc. | $N$, $(o_1, o_2)$ | $K$ | $n_{\mathrm{H}}$ | $n_{\mathrm{C}}$ | Acc. |
|---|---|---|---|---|---|---|---|---|---|---|---|---|---|---|
| $10^2$, (4,2) | 2 | 2 | 10 | 0.683(7) | $10^3$, (6,2) | 2 | 2 | 10 | 0.823(6) | $10^4$, (8,2) | **2** | 2 | 10 | 0.362(1) |
| | | | 20 | 0.713(8) | | | | 20 | 0.829(2) | | | | 20 | 0.39(3) |
| | | 4 | 10 | 0.769(6) | | | 4 | 10 | 0.830(5) | | | **4** | **10** | **0.860(7)** |
| | | | 20 | 0.778(3) | | | | 20 | 0.81(1) | | | | 20 | 0.75(9) |
| | **4** | 2 | 10 | 0.752(3) | | **4** | 2 | 10 | 0.814(8) | | 4 | 2 | 10 | 0.48(7) |
| | | | 20 | 0.762(5) | | | | 20 | 0.825(5) | | | | 20 | 0.71(9) |
| | | **4** | 10 | 0.802(8) | | | **4** | 10 | 0.853(3) | | | 4 | 10 | 0.85(1) |
| | | | **20** | **0.83(1)** | | | | **20** | **0.860(7)** | | | | 20 | $\cdots$ |

Table S4: Evaluation accuracies for off-lattice connectivity percolation data varying the meta-parameters, with $N$ the number of particles and $(o_1, o_2)$ the overweighting factors for class 1 and 2 respectively. The '$\cdots$' for $N = 10^4$ denotes training was not possible on the production system.

| Classification | $L$ | Spectral GNN | Standard GNN | Edges | Positions | Edges and Positions |
|---|---|---|---|---|---|---|
| | 20 | 0.930(5) | 0.542(1) | 0.935(5) | 0.938(5) | 0.926(4) |
| Rigidity | 50 | 0.953(3) | 0.538(1) | 0.943(9) | 0.943(7) | 0.945(5) |
| | 100 | 0.975(5) | 0.522(1) | 0.966(7) | 0.974(4) | 0.980(4) |
| | 20 | 0.790(3) | 0.447(1) | 0.785(5) | 0.795(5) | 0.792(6) |
| Connectivity | 50 | 0.902(2) | 0.491(1) | 0.902(2) | 0.900(3) | 0.901(2) |
| | 100 | 0.861(6) | 0.2(1) | 0.85(1) | 0.869(5) | 0.87(1) |

Table S5: Accuracies for different model and data variations for both rigidity and classification problems on the lattice, with the same meta-parameters as Figs. 1 and 2 in the main text. Spectral GNN refers to the Chebyshev filtering model of [2] and standard GNN refers for a graph neural network with normal message passing [1]. The remaining columns refer to additional features in the data set, either for the edges (scalar separation between nodes), the nodes ($(x, y)$ coordinates), and both together.

| Classn | $N$ | Spectral GNN | GNN | Edges | Positions | Edges+Pos. | Max. Clust. |
|---|---|---|---|---|---|---|---|
| | $10^2$ | 0.870(4) | 0.664(1) | 0.863(4) | 0.865(8) | 0.854(7) | 0.846(6) |
| Rigidity | $10^3$ | 0.868(8) | 0.570(1) | 0.869(2) | 0.864(4) | 0.868(6) | 0.837(8) |
| | $10^4$ | 0.748(7) | 0.554(1) | 0.746(7) | 0.748(7) | 0.754(5) | 0.67(5) |
| | $10^2$ | 0.83(1) | 0.168(1) | 0.741(8) | 0.746(2) | 0.755(5) | 0.658(6) |
| Conn. | $10^3$ | 0.860(7) | 0.640(1) | 0.828(4) | 0.830(7) | 0.817(5) | 0.749(6) |
| | $10^4$ | 0.860(7) | 0.362(1) | 0.84(1) | 0.863(8) | 0.86(1) | 0.77(2) |

Table S6: Accuracies for different model and data variations for both rigidity and classification problems for the off-lattice data. Other details as per Table S5.
